# Supplementary material for: Neural Parameter Allocation Search
Source: arXiv:2006.10598 source file (2022-03-16)
Supplement: Supplementary file 1 [file supp_2_results_std.tex]

\section{Results with Standard Deviation}
\label{sec:results_std}
The results in our paper are averaged over five runs, except ImageNet which was averaged over three.  In this section we provide standard deviations for our results, which we could not provide in our paper due to space constraints.   This includes bidirectional image-sentence retrieval (Table~\ref{tab:ret_std}), phrase grounding (Table~\ref{tab:ground_std}), image classification (Table~\ref{tab:cls_std}), and knowledge distillation (Table~\ref{tab:distill_std}).  The inclusion of standard deviation helps to solidify the significance of our reported performance gains using SSNs.

\begin{table}[!htbp]
    \centering
    \caption{Bidirectional image-sentence retrieval results with standard deviations from Table 1 and Table 2 from our paper.  Please refer to our paper for number of parameters and groups used for each experiment. Note that  ``Baseline'' refers to using with no parameter sharing, and ``Reduced Baseline'' adjusts the number and/or size of filters of the baseline so they have the same number of parameters as our SSNs.}
    \begin{tabular}{lcccc}
    \toprule
    Architecture & \multicolumn{2}{c}{EmbNet~\cite{Wang_2016_CVPR}} & \multicolumn{2}{c}{ADAPT-T2I~\cite{Wehrmann_2020_AAAI}}\\
    \midrule
    Dataset & F30K~\cite{young2014image} & MSCOCO~\cite{lin2014microsoft} & F30K~\cite{young2014image} & MSCOCO~\cite{lin2014microsoft}\\ 
    \midrule
    \multicolumn{3}{l}{\textbf{Parameter Combiner Comparison}} \\
    \midrule
    Reduced Baseline & 72.8 $\pm$ 0.19 & 80.9 $\pm$ 0.26 & 80.6 $\pm$ 0.15 & 85.2 $\pm$ 0.16\\
    RR & 74.1 $\pm$ 0.25 & 80.8 $\pm$ 0.25 & 81.2 $\pm$ 0.18 & 85.6 $\pm$ 0.18 \\
    Avg & 73.5 $\pm$ 0.21 & 80.9 $\pm$ 0.28 & 80.5 $\pm$ 0.23 & 85.8 $\pm$ 0.21 \\
    WAvg & 74.0 $\pm$ 0.18 & 81.2 $\pm$ 0.22 & 81.6 $\pm$ 0.21 & \textbf{86.2 $\pm$ 0.23}\\
    Emb & \textbf{74.3 $\pm$ 0.27} & \textbf{81.5 $\pm$ 0.32} & \textbf{81.7 $\pm$ 0.19} & 85.9 $\pm$ 0.32\\
    \midrule
        \multicolumn{4}{l}{\textbf{Parameter Bank Grouping Comparison}} \\
        \midrule
        Baseline & 74.1 $\pm$ 0.33 & 81.4 $\pm$ 0.31 & \textbf{83.3 $\pm$ 0.21} & 86.8 $\pm$ 0.17\\
        Single & \textbf{74.4 $\pm$ 0.26} & \textbf{82.1 $\pm$ 0.26} & 82.1 $\pm$ 0.16 & 86.1 $\pm$ 0.19\\
        Random & 74.0 $\pm$ 0.36 & 81.5 $\pm$ 0.25 & 81.9 $\pm$ 0.28 & 86.3 $\pm$ 0.25\\
        Manual & 74.3 $\pm$ 0.24 & 81.7 $\pm$ 0.29 & 82.0 $\pm$ 0.20 & 86.1 $\pm$ 0.21\\
        WAvg & 74.2 $\pm$ 0.23 & 81.7 $\pm$ 0.25 & 82.6 $\pm$ 0.20 & 86.4 $\pm$ 0.17\\
        Emb & 74.3 $\pm$ 0.14 & 81.9 $\pm$ 0.30 & 82.9 $\pm$ 0.22 & \textbf{87.0 $\pm$ 0.23}\\
        \bottomrule
    \end{tabular}
    \label{tab:ret_std}
\end{table}

\begin{table}[!htbp]
    \centering
    \caption{Phrase grounding results with standard deviations from Table 1 and Table 2 from our paper.  Please refer to our paper for number of parameters and groups used for each experiment. Note that  ``Baseline'' refers to using no parameter sharing, and ``Reduced Baseline'' adjusts the number and/or size of filters of the baseline so they have the same number of parameters as our SSNs.}
    \begin{tabular}{lcc}
    \toprule
    Architecture & \multicolumn{2}{c}{SimNet~\cite{wang2018learning}} \\
    \midrule
    Dataset & F30K Entities~\cite{flickrentitiesijcv} & ReferIt~\cite{kazemzadeh-EtAl:2014:EMNLP2014}\\ 
    \midrule
    \multicolumn{3}{l}{\textbf{Parameter Combiner Comparison}} \\
    \midrule
    Reduced Baseline & 71.1 $\pm$ 0.28 & 59.4 $\pm$ 0.49\\
    RR & 72.3 $\pm$ 0.28 & \textbf{60.5 $\pm$ 0.53}\\
    Avg & 72.1 $\pm$ 0.31 & 60.2 $\pm$ 0.53\\
    WAvg & 72.3 $\pm$ 0.25 & \textbf{60.5 $\pm$ 0.48}\\
    Emb & \textbf{72.5 $\pm$ 0.30} & 60.4 $\pm$ 0.52\\
    \midrule
        \multicolumn{3}{l}{\textbf{Parameter Bank Grouping Comparison}} \\
        \midrule
        Baseline & 71.7 $\pm$ 0.26 & \textbf{61.1 $\pm$ 0.39}\\
        Single & 71.4 $\pm$ 0.33 & 60.9 $\pm$ 0.56\\
        Random & 71.8 $\pm$ 0.43 & 60.0 $\pm$ 0.57\\
        Manual & \textbf{72.4 $\pm$ 0.29} & 60.2 $\pm$ 0.49\\
        WAvg & 72.2 $\pm$ 0.34 & 61.0 $\pm$ 0.43\\
        Emb & 72.1 $\pm$ 0.28 & 60.5 $\pm$ 0.57\\
        \bottomrule
    \end{tabular}
    \label{tab:ground_std}
\end{table}

\begin{table}[!htbp]
    \centering
    \caption{Image classification results with standard deviations from Table 1 and Table 2 from our paper.  Please refer to our paper for number of parameters and groups in each experiment. Note that  ``Baseline'' refers to using no parameter sharing, and ``Reduced Baseline'' adjusts the number and/or size of filters of the baseline so they have the same number of parameters as our SSNs.}
    \begin{tabular}{lccc}
    \toprule
    Architecture & \multicolumn{2}{c}{WRN-28-10~\cite{Zagoruyko2016WRN}} & WRN-50-2~\cite{Zagoruyko2016WRN}\\
    \midrule
    Dataset & CIFAR-10~\cite{cifar} & CIFAR-100~\cite{cifar} & ImageNet~\cite{deng2009imagenet}\\ \midrule
    \multicolumn{3}{l}{\textbf{Parameter Combiner Comparison}} \\
    \midrule
    Reduced Baseline & 4.22 $\pm$ 0.16 & 22.34 $\pm$ 0.12 & 10.08 $\pm$ 0.02\\
    RR & 4.09 $\pm$ 0.34 & 21.91 $\pm$ 0.24 & \textbf{6.69 $\pm$ 0.08}\\
    Avg & 4.19 $\pm$ 0.11 & 22.78 $\pm$ 0.29 & 7.61 $\pm$ 0.07\\
    WAvg & 4.00 $\pm$ 0.08 & \textbf{21.78 $\pm$ 0.26} & 7.38 $\pm$ 0.02\\
    Emb & \textbf{3.84 $\pm$ 0.13} & 21.92 $\pm$ 0.30 & \textbf{6.69 $\pm$ 0.11}\\
    \midrule
        \multicolumn{4}{l}{\textbf{Parameter Bank Grouping Comparison}} \\
        \midrule
        Baseline & 3.57 $\pm$ 0.19 & 19.44 $\pm$ 0.21 & 5.84 $\pm$ 0.06\\
        Single & 3.71 $\pm$ 0.17 & 19.99 $\pm$ 0.22 & 6.18 $\pm$ 0.05\\
        Random & 3.63 $\pm$ 0.11 & 20.36 $\pm$ 0.50 & 5.91 $\pm$ 0.08\\
        Manual & \textbf{3.38 $\pm$ 0.14} & 19.29 $\pm$ 0.26 & \textbf{5.82 $\pm$ 0.01}\\
        WAvg & 3.51 $\pm$ 0.11 & 19.47 $\pm$ 0.30 & 5.86 $\pm$ 0.06\\
        Emb & 3.42 $\pm$ 0.06 & \textbf{19.24 $\pm$ 0.29} & 5.96 $\pm$ 0.06\\
        \bottomrule
    \end{tabular}
    \label{tab:cls_std}
\end{table}

\begin{table}[!htbp]
    \centering
    \caption{Experimental setup for our knowledge distillation experiments reported in Table~\ref{tab:distill_std}.}
    \begin{tabular}{cccccc}
    \toprule
    Experiment & Teacher & \#Params (M) & Student  & \#Params (M) & Dataset\\
    \midrule
        (a) & WRN-28-4 & 5.87 & WRN-28-2 & 1.47 & CIFAR-100\\
        (b) & WRN-28-4 & 5.87 & WRN-16-2 & 0.70 & CIFAR-100\\
    \bottomrule
    \end{tabular}
    \label{tab:distill_setup}
\end{table}

\begin{table}[!htbp]
    \centering
    \caption{Knowledge distillation results with standard deviation on CIFAR-100 using teacher/student setup in Table~\ref{tab:distill_setup}.  Note our SSNs only use a teacher network when combined with OD~\cite{Heo_2019_ICCV}.  See Section 4.3 of our paper for discussion.}
    \setlength{\tabcolsep}{2pt}
    \begin{tabular}{cccccccccccc}
    \toprule
    Experiment & Teacher & Baseline & AT~\cite{Zagoruyko2017AT} & Jacobian~\cite{SrinivasJacobianICML2018} & FT~\cite{kimFactorTransfer2018} & AB~\cite{ABdistill} & OD~\cite{Heo_2019_ICCV} & SSN (ours) & SSN+OD\\
    \midrule
        (a) & 21.09 & 24.88 & 23.80 & 23.70 & 23.41 & 23.19 & 21.98 & 23.62 $\pm$ 0.13 & \textbf{21.21 $\pm$ 0.21}\\
        (b) & 21.09 & 27.32 & 26.56 & 26.71 & 25.91 & 26.02 & 24.08 & 26.53 $\pm$ 0.15 & \textbf{23.30 $\pm$ 0.19}\\
    \bottomrule
    \end{tabular}
    \label{tab:distill_std}
\end{table}

%\clearpage
