# Supplementary material for: Neural Parameter Allocation Search
Source: arXiv:2006.10598 source file (2022-03-16)
Supplement: Supplementary file 2 [file supp_0_main.tex]

\documentclass[10pt,twocolumn,letterpaper]{article}

\usepackage{iccv}
\usepackage{times}
\usepackage{epsfig}
\usepackage{graphicx}
\usepackage{amsmath}
\usepackage{amssymb}
\usepackage{microtype}

\usepackage{xspace}
\usepackage{multirow}
\usepackage{color}
\usepackage{svg}
\usepackage{cite}
\usepackage{booktabs}

% Include other packages here, before hyperref.

% If you comment hyperref and then uncomment it, you should delete
% egpaper.aux before re-running latex.  (Or just hit 'q' on the first latex
% run, let it finish, and you should be clear).
\usepackage[pagebackref=true,breaklinks=true,letterpaper=true,colorlinks,bookmarks=false]{hyperref}

% \iccvfinalcopy % *** Uncomment this line for the final submission

 % *** Enter the ICCV Paper ID here

% Pages are numbered in submission mode, and unnumbered in camera-ready
\ificcvfinal\pagestyle{empty}\fi

\begin{document}

%%%%%%%%% TITLE
\title{Neural Parameter Allocation Search}

\author{First Author\\
Institution1\\
Institution1 address\\
{\tt\small firstauthor@i1.org}
% For a paper whose authors are all at the same institution,
% omit the following lines up until the closing ``}''.
% Additional authors and addresses can be added with ``\and'',
% just like the second author.
% To save space, use either the email address or home page, not both
\and
Second Author\\
Institution2\\
First line of institution2 address\\
{\tt\small secondauthor@i2.org}
}

\maketitle
% Remove page # from the first page of camera-ready.
\ificcvfinal\thispagestyle{empty}\fi
\input{supp_1_models}
\input{supp_3_baselines}
\input{supp_4_group}
\input{supp_5_bank}
\input{supp_6_figure}

{\small
\bibliographystyle{ieee_fullname}
\bibliography{egbib}
}

\end{document}
